# Supplementary material for: Online Sign Identification: Minimization of the Number of Errors in Thresholding Bandits
Source: arXiv:2110.09133 source file (2021-10-18)
Supplement: Supplementary file 1 [file APT_proof.tex]

% !TeX root = ../neurips_2021.tex
\section{APT}
\label{app:apt}

We provide an upper bound on the expected loss of APT for the zero-one loss, following the method of \cite{locatelli2016optimal}, but with a greater care for the constant factors in the exponential.

The algorithm we analyze is the generalization of APT to one-parameter exponential families, which pulls $k_t = \argmin_{k\in[K]} N_{t-1}^k \KL(\hat{\mu}_{t-1}^k, \theta)$.

\begin{theorem}
The expected loss of the APT algorithm on the zero-one loss setting is
\begin{align*}
\mathbb{E}[L_T] \le KT \exp\left( - \frac{T - K}{H}\right) \: ,
\end{align*}
where $H = \sum_{k=1}^K \frac{1}{\text{ch}(\mu_k, \theta)}$, with $\text{ch}(\mu_k, \theta) = \min_{x \in \mathbb{R}} \max \{\KL(x, \mu_k), \KL(x, \theta)\}$.
\end{theorem}
For Gaussian distributions with variance $\sigma^2$, $\text{ch}(\mu_k, \theta) = \frac{1}{4} \KL(\mu_k, \theta) = \frac{1}{4}\frac{\Delta_k^2}{2 \sigma^2}$ . Note that the bound obtained for Gaussian distributions is also valid for sub-Gaussians.

The factor $T$ in front of the exponential is worse than the $\log T$ of \cite{locatelli2016optimal}. It is due to the use of a coarser union bound.

\begin{proof}
The three pillars of the proof are:
\begin{itemize}
\item If arm $k$ is pulled at time $t$, for all $j \in [K]$,
\begin{align*}
N_{t-1}^j \KL(\hat{\mu}_{t-1}^j, \theta) \ge N_{t-1}^k \KL(\hat{\mu}_{t-1}^k, \theta) \: .
\end{align*}
\item If there is a mistake on arm $j$ after $t$,
\begin{align*}
N_t^j \KL(\hat{\mu}_t^j, \mu^j) \ge N_t^j \KL(\hat{\mu}_t^j, \theta) + N_t^j \KL(\theta, \mu^j) \: .
\end{align*}
\item With probability $1 - \delta$, for all $j \in [K]$ and all $t \in [T]$,
\begin{align*}
N_t^j \KL(\hat{\mu}_t^j, \mu^j) < \log \frac{KT}{\delta} \: .
\end{align*}
\end{itemize}

Let $\text{ch}(\mu_k, \theta) = \min_x \max \{\KL(x, \mu_k), \KL(x, \theta)\}$ and $H = \sum_{k=1}^K \frac{1}{\text{ch}(\mu_k, \theta)}$.
At time $T$, there exists $k \in [K]$ such that $N_T^k - 1 \ge \frac{T - K}{H \text{ch}(\mu_k, \theta)}$, since the sum over $k$ of the two sides is the same.

At the last time at which that $k$ was pulled we had $N_{t-1}^k = N_T^k - 1$. At that time, for all $j$ for which there is a mistake,
\begin{align*}
N_{t-1}^j \KL(\hat{\mu}_{t-1}^j, \mu^j)
\ge N_{t-1}^j \KL(\hat{\mu}_{t-1}^j, \theta)
\ge N_{t-1}^k \KL(\hat{\mu}_{t-1}^k, \theta)
&\ge \frac{T - K}{H \text{ch}(\mu_k, \theta)} \KL(\hat{\mu}_{t-1}^k, \theta)
\: .
\end{align*}

With probability $1 - \delta$,
\begin{align*}
\KL(\hat{\mu}_{t-1}^k, \mu^k) \le \frac{H\text{ch}(\mu_k, \theta)}{T-K}\log \frac{KT}{\delta}
\: .
\end{align*}
For $\delta = KT \exp\left( - \frac{T - K}{H}\right)$, we get $\KL(\hat{\mu}_{t-1}^k, \mu^k) \le \text{ch}(\mu_k, \theta)$, with consequence that $\KL(\hat{\mu}_{t-1}^k,\theta) \ge \text{ch}(\mu_k, \theta)$.
Then for all $j$ such that there is a mistake,
\begin{align*}
N_{t-1}^j \KL(\hat{\mu}_{t-1}^j, \mu^j)
&\ge \frac{T - K}{H}
= \log \frac{KT}{\delta}
\: .
\end{align*}
This is in contradiction with the concentration event. We conclude that with probability $1 - KT \exp\left( - \frac{T - K}{H}\right)$, there is no mistake at that time $t$.
\end{proof}
